# Supplementary material for: T-RECX: Tiny-Resource Efficient Convolutional neural networks with early-eXit
Source: arXiv:2207.06613 source file (2023-04-26)
Supplement: Supplementary file 1 [file appendix.tex]

% LaTeX template for Artifact Evaluation V20201122
%
% Prepared by Grigori Fursin with contributions from Bruce Childers,
%   Michael Heroux, Michela Taufer and other colleagues.
%
% See examples of this Artifact Appendix in
%  * SC'17 paper: https://dl.acm.org/citation.cfm?id=3126948
%  * CGO'17 paper: https://www.cl.cam.ac.uk/~sa614/papers/Software-Prefetching-CGO2017.pdf
%  * ACM ReQuEST-ASPLOS'18 paper: https://dl.acm.org/citation.cfm?doid=3229762.3229763
%
% (C)opyright 2014-2022
%
% CC BY 4.0 license
%

% \documentclass{sigplanconf}

% \usepackage{hyperref}

% \begin{document}

% \special{papersize=8.5in,11in}

%%%%%%%%%%%%%%%%%%%%%%%%%%%%%%%%%%%%%%%%%%%%%%%%%%%%
% When adding this appendix to your paper, 
% please remove above part
%%%%%%%%%%%%%%%%%%%%%%%%%%%%%%%%%%%%%%%%%%%%%%%%%%%%

\appendix
\section{Artifact Appendix}

%%%%%%%%%%%%%%%%%%%%%%%%%%%%%%%%%%%%%%%%%%%%%%%%%%%%%%%%%%%%%%%%%%%%%
\subsection{Abstract}
This appendix describes the artifact associated with this work.
\subsection{Artifact meta-information}

% {\em Obligatory. Use just a few informal keywords in all fields applicable to your artifacts
% and remove the rest. This information is needed to find appropriate reviewers and gradually 
% unify artifact meta information in Digital Libraries.}

{\small
\begin{itemize}
  \item {\bf Algorithm:} Early-exit technique for tinyCNNs
  \item {\bf Program:} Tensorflow v2.3
  \item {\bf Compilation:} Python v3.7, Tensorflow v2.3
  \item {\bf Model:} Resnet-8, DSCNN, MobinetV1
  \item {\bf Datasets:} CIFAR-10, Speech Commands, Visual wake words
  \item {\bf Run-time environment:} Ubuntu Linux with miniconda
  \item {\bf Hardware:} GeForce RTX 2080 GPU for model training 
  \item {\bf Run-time state:} set by our scripts
  \item {\bf Metrics: }prediction accuracy, FLOPS
  \item {\bf Output: } Accuracy vs FLOPS trade-off plot (benefit curve)
  \item {\bf How much disk space required (approximately)?: } $\sim$15GB
  \item {\bf How much time is needed to prepare workflow?: }30-40min
  \item {\bf How much time is needed to complete experiments?: }Several hours. Each model takes around 4 to 5 hours to train on a GPU. Testing on either trained models (or on pretrained models included in artifact) takes $\sim$45-60min 
  \item {\bf Publicly available?: }Yes. Datasets are also publicly available
\end{itemize}
}

%%%%%%%%%%%%%%%%%%%%%%%%%%%%%%%%%%%%%%%%%%%%%%%%%%%%%%%%%%%%%%%%%%%%%
\subsection{Description}

\subsubsection{How to access}
\url{https://github.com/nikhilghanathe/t-recx}

\subsubsection{Hardware dependencies}
The results reported are based on training done on a GeForce RTX 2080 GPU. The workflow can practically be run on any laptop/desktop with a GPU.

\subsubsection{Software dependencies}
Ubuntu Linux, Tensorflow=2.3, Cudatoolkit=10.1, Cudnn=7.6, Python=3.7. Other tested build configurations for tensorflow can be found at: \url{https://www.tensorflow.org/install/source#gpu}

%%%%%%%%%%%%%%%%%%%%%%%%%%%%%%%%%%%%%%%%%%%%%%%%%%%%%%%%%%%%%%%%%%%%%
\subsection{Installation}
\tool uses miniconda package manager. Installation instructions for Linux at: \url{https://docs.conda.io/en/latest/miniconda.html}

\vspace{1mm}\noindent
\emph{Prepare environment}

    \noindent\texttt{\$ conda create -n trecx python=3.7}
    
    \noindent\texttt{\$ conda activate trecx}

\vspace{1mm}\noindent
\emph{Clone repository and run install script}

    \noindent\texttt{\$ git clone https://github.com/nikhilghanathe/t-recx.git}

    \noindent\texttt{\$ bash install\_conda\_packages.sh}
    
    \noindent\texttt{\$ pip install -r requirements.txt}

%%%%%%%%%%%%%%%%%%%%%%%%%%%%%%%%%%%%%%%%%%%%%%%%%%%%%%%%%%%%%%%%%%%%%
\subsection{Experiment workflow}
The repository contains three directories: image\_classification, keyword\_spotting, visual\_wake\_words. These directories correspond to evaluation of 1)~Resnet-8 on CIFAR-10, 2)~DSCNN on Speech Commands and 3)~MobilenetV1 on Visual wake words datasets respectively. The scripts for downloading datasets, preprocessing, training and testing have all been automated, and are included in each directory. The scripts included use model hyperparameters and architectures described in this paper. More details can be found in the \texttt{README.md} file in each directory. 

The repository also contains pretrained models. As an alternative to several hours of training, the results presented in this work can be verified by running the test script included in each directory. Details on running the test scripts can be found in the corresponding \texttt{README.md} files.
%%%%%%%%%%%%%%%%%%%%%%%%%%%%%%%%%%%%%%%%%%%%%%%%%%%%%%%%%%%%%%%%%%%%%
\subsection{Evaluation and expected results}
The output from running the test scripts in each directory on the trained models is saved in the \texttt{results/} sub-directory. The test script generates the benefit curve plots of Figure~\ref{fig:benefit_curve}, Figure~\ref{fig:benefit_curve_prior} and Figure~\ref{fig:benefit_curve_ev} of the paper.

%%%%%%%%%%%%%%%%%%%%%%%%%%%%%%%%%%%%%%%%%%%%%%%%%%%%%%%%%%%%%%%%%%%%%
% \subsection{Experiment customization}

%%%%%%%%%%%%%%%%%%%%%%%%%%%%%%%%%%%%%%%%%%%%%%%%%%%%%%%%%%%%%%%%%%%%%
% \subsection{Notes}

% %%%%%%%%%%%%%%%%%%%%%%%%%%%%%%%%%%%%%%%%%%%%%%%%%%%%%%%%%%%%%%%%%%%%%
% \subsection{Methodology}

% Submission, reviewing and badging methodology:

% \begin{itemize}
%   \item \url{https://docs.conda.io/projects/conda/en/latest/user-guide/install/linux.html}
%   \url{https://www.acm.org/publications/policies/artifact-review-badging}
%   \item \url{http://cTuning.org/ae/submission-20201122.html}
%   \item \url{http://cTuning.org/ae/reviewing-20201122.html}
% \end{itemize}

%%%%%%%%%%%%%%%%%%%%%%%%%%%%%%%%%%%%%%%%%%%%%%%%%%%%
% When adding this appendix to your paper, 
% please remove below part
%%%%%%%%%%%%%%%%%%%%%%%%%%%%%%%%%%%%%%%%%%%%%%%%%%%%

% \end{document}
